# Supplementary material for: Distance Preserving Graph Simplification
Source: arXiv:1110.0517 source file (2011-10-03)
Supplement: Supplementary file 1 [file Appendix.tex]

\subsection{Appendix}
\label{apps}

\input{Figures/GatesDiscovery.tex}

The overall procedure to discover gate is outlined in Algorithm \ref{alg:gatesdiscovery}.
We use $V^\ast$ to store the resulting {\em gates}, and $R$ to record the set of the set of vertex pairs which has been covered during the procedure.
The procedure starts with initializing $V\ast$ and $R$ to be empty set (Line 1 and Line 2).
Then, breath-first-search (BFS) traversal is employed $|V|$ times to gain all vertex pairs whose shortest distance is $\epsilon+1$.
During the procedure of BFS, the ground set $S$ recording all vertex pairs with distance $\epsilon+1$ is collected,
and each vertex $v$'s associated set $S_v$ is also updated (Line 3 to Line 5).
In the while loop for greedy cover (Line 6 to Line 10), for each iteration, we always choose an unselected vertex $v$ such that $\frac{1}{S_v \cap (S \setminus R)}$ is minimum (Line 7).
In the meanwhile, $V^\ast$ and $R$ are also updated (Line 8 to Line 9).
This procedure repeats until all vertex pairs are covered in $R$ and the resulting gates are stored in $V^\ast$.
